# Supplementary material for: Causal-based Time Series Domain Generalization for Vehicle Intention Prediction
Source: arXiv:2112.02093 source file (2021-12-03)
Supplement: Supplementary file 7 [file Reference.tex]

\subsection*{References}

[1] S. Tople, A. Sharma, and A. Nori.  Alleviating privacy attacks via causal learning.  In \textit{International Conference on Machine Learning}, pages 9537–9547. PMLR, 2020.
